# Supplementary material for: Assessing the Scalability of Biologically-Motivated Deep Learning Algorithms and Architectures
Source: arXiv:1807.04587 source file (2018-11-20)
Supplement: Supplementary file 1 [file appendix_padding_dim.tex]

\subsection{Auxiliary output size effect on AO-SDTP}
